# Supplementary material for: Localised vibrations in superconducting YBCO revealed by ultra-fast optical coherent spectroscopy
Source: arXiv:1408.0888 source file (2017-11-06)
Supplement: Supplementary file 1 [file Supplementary.pdf]

# Online supplementary information: Dynamical coupling between off-plane phonons and in-plane electronic excitations in superconducting YBCO

Daniele Fausti,[1,2] Fabio Novelli,[2] Gianluca Giovannetti,[3] Adolfo Avella,[4,5]
Federico Cilento,[2] Milan Radovic,[6,7] Massimo Capone,[3] and Fulvio Parmigiani[8,2]

[1] *Department of Physics, Universit degli Studi di Trieste, 34127 Trieste, Italy*
[2] *Sincrotrone Trieste SCpA, 34127 Basovizza, Italy**
[3] *CNR-IOM Democritos National Simulation Center and Scuola Internazionale Superiore di Studi Avanzati (SISSA), Via Bonomea 265, 34136 Trieste, Italy*
[4] *Dipartimento di Fisica "E.R. Caianiello" - UnitàCNISM di Salerno, Università degli Studi di Salerno, I-84084 Fisciano (SA), Italy*
[5] *CNR-SPIN, UoS di Salerno, I-84084 Fisciano (SA), Italy*
[6] *Swiss Light Source, Paul Scherrer Institute, CH-5232 Villigen PSI, Switzerland*
[7] *Institut de la Matiere Complexe, EPF Lausanne, CH-1015 Lausanne, Switzerland*
[8] *Department of Physics, Università degli Studi di Trieste, 34127 Trieste, Italy*

(Dated: July 31, 2014)

PACS numbers: Valid PACS appear here

* daniele.fausti@elettra.eu

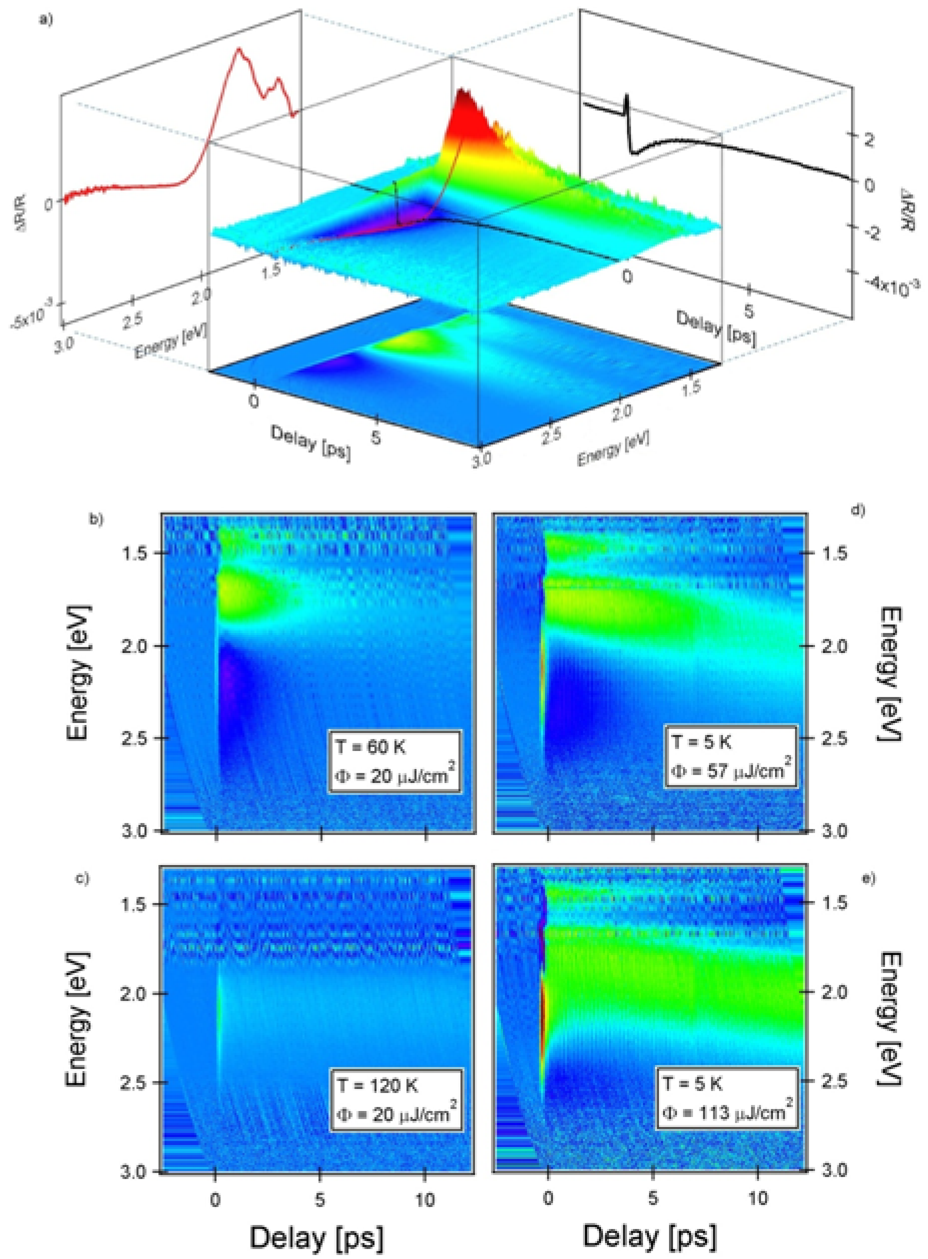


FIG. 1. Representative measurements for the time domain reflectivity as a function of the probe wavelength and time delay between pump and probe. Fig. a and b are representative for low fluence low temperature, fig. c for low fluence high temperature (c), and d and e for high fluence low temperature. The measurement in a is performed at 5K with pump fluence of $20\mu\mathrm{J/cm}^2$, while the temperature and fluence for the other measurements are indicated in the insert of each panel.
